# Supplementary material for: Mechanisms for a No-Regret Agent: Beyond the Common Prior
Source: arXiv:2009.05518 source file (2020-09-11)
Supplement: Supplementary file 1 [file appendixC6.tex]

\begin{lemma}\label{L9}
	Let $B\subseteq [0,1]$ and $\Pi\subseteq\Delta(\mathcal{Y})$ be finite sets. Suppose the principal uses a mechanism $\sigma^*$ that draws $p\sim\diamondsuit$ uniformly with probability $\alpha$, and with probability $1-\alpha$ mixes over the buffered policies $p^\dagger(b,\pi)$ for $b\in B$, $\pi\in\Pi$. Then there exists a learner $L$ that guarantees
	\[
	\er{\Delta(\mathcal{Y})}\leq\sqrt{2T |B||\Pi|\log|\mathcal{R}|}+\alpha\left(K_\spadesuit+TB_U\sqrt{\frac{|\mathcal{Y}|\log T}{2T}}\right)
	\]
\end{lemma}
\begin{proof}
	For each $\vec{r}\in\mathcal{R}^{B\times\Pi}$, define a set of beliefs that respond to $p^\dagger(\pi,b)$ with $\vec{r}(b,\pi)$:
	\[
	\Pi_{\vec{r}}=\left\{\pi\in\Delta(\mathcal{Y})\mid \vec{r}\in\left(r_\pi(p(b,\tilde\pi))\right)_{b\in B,\tilde{\pi}\in\Pi}\right\}
	\]
	\textcite{KBTB15} defined a generalized Hedge algorithm as follows. Let $\mu_0$ be an initial distribution over $\Pi_{\vec{r}}$. Define
	\[
	\mu_{t+1,\vec{r}}(\pi)\propto\mu_{0,\vec{r}}(\pi)\cdot\exp\left(\eta\sum_{i=1}^t\ex[p\sim\diamondsuit]{U(\pi,p,y_t)}\right)\quad\mathrm{where}\quad\eta=\frac{1}{B_U}\sqrt{\frac{8|\mathcal{Y}|\log T}{T}}
	\]
	The set $\Pi_{\vec{r}}\subseteq\Delta(\mathcal{Y})\subseteq\reals^\mathcal{Y}$ is convex, compact, with diameter less than one. By the second part of assumption \ref{A12}, the function $\ex[p\sim\diamondsuit]{U(\pi,p,y)}$ is equi-Lipschitz continuous in $\pi$ where $K_\spadesuit$ is the Lipschitz constant. By corollary 2 of \textcite{KBTB15}, this algorithm attains regret
	\begin{equation}\label{E40}
	\sum_{t=1}^T\left(\ex[p\sim\diamondsuit]{U(\pi_0,p,y_t)}-\ex[\pi\sim\mu_{t,\vec{r}_0}]{\ex[p\sim\diamondsuit]{U(\pi,p,y_t)}}\right)
	\leq K_\spadesuit+TB_U\sqrt{\frac{|\mathcal{Y}|\log T}{2T}}
	\end{equation}
	for any $\pi_0\in\Pi_{\vec{r}}$. Thus, for any choice of $\vec{r}_t$, the generalized Hedge algorithm recommends a distribution $\mu_{t,\vec{r}}\in\Delta(\Pi_{\vec{r}})$ over priors that induce $\vec{r}$. We can regard this as a (finite) set of experts, with respect to which the exponential weights algorithm (see e.g. \cite{CL06}) guarantees
	\begin{align*}
		&(1-\alpha)\sum_{t=1}^T\left(\ex[b,\pi\sim\upsilon_t]{U(\vec{r}_0(b,\pi),p^\dagger(b,\pi),y_t)}-\ex[\vec{r}\sim F]{\ex[b,\pi\sim\upsilon_t]{U(\vec{r}(b,\pi),p^\dagger(b,\pi),y_t)}}\right)\\
		&\:\:\:\:+\alpha\sum_{t=1}^T\left(\ex[\pi\sim\mu_{t,\vec{r}_0}]{\ex[p\sim\diamondsuit]{U(\pi,p,y_t)}}-\ex[\vec{r}\sim F]{\ex[\pi\sim\mu_{t,\vec{r}}]{\ex[p\sim\diamondsuit]{U(\pi,p,y_t)}}}\right)\\
		&\leq\sqrt{2T |B||\Pi|\log|\mathcal{R}|}
	\end{align*}
	for any $\vec{r}_0$. Combining this with the earlier bound \eqref{E40}, it follows that for any $\pi_0\in\Pi_{\vec{r}_0}$,
	\begin{align*}
		&(1-\alpha)\sum_{t=1}^T\left(\ex[b,\pi\sim\upsilon_t]{U(\vec{r}_0(b,\pi),p^\dagger(b,\pi),y_t)}-\ex[\vec{r}\sim F]{\ex[b,\pi\sim\upsilon_t]{U(\vec{r}(b,\pi),p^\dagger(b,\pi),y_t)}}\right)\\
		&\:\:\:\:+\alpha\sum_{t=1}^T\left(\ex[p\sim\diamondsuit]{U(\pi_0,p,y_t)}-\ex[\vec{r}\sim F]{\ex[\pi\sim\mu_{t,\vec{r}}]{\ex[p\sim\diamondsuit]{U(\pi,p,y_t)}}}\right)\\
		&\leq\sqrt{2T |B||\Pi|\log|\mathcal{R}|}+\alpha\left(K_\spadesuit+TB_U\sqrt{\frac{|\mathcal{Y}|\log T}{2T}}\right)
	\end{align*}
	This was the desired result.
\end{proof}

The following proposition presents a no-contextual-regret algorithm for the agent, which includes as special cases no-CIR and no-PCIR algorithms.

\begin{prop}\label{P5}
	Let $\mathcal{D}_{\vec{r}}$ be a partition of $\Pi_{\vec{r}}$ where $d(\pi,\Pi_{\vec{r}})\leq\delta$ for any $\pi\in\Pi_{\vec{r}}$. Let $\mathcal{D}=\bigcup_{\vec{r}}\mathcal{D}_{\vec{r}}$. Consider the set $\mathcal{G}$ of all modification rules $G:\mathcal{C}\to\mathcal{D}$. Consider the same class of mechanisms $\sigma^*$ described in lemma \ref{L9}. Then there exists a learner $L$ whose contextual regret is at most
	\[
	\sqrt{2T |B||\Pi|\log|\mathcal{R}|}+\alpha\left(K_\spadesuit(1+\delta T)+TB_U\sqrt{\frac{|\mathcal{Y}|\log T}{2T}}\right)+O\left(\sqrt{T|\mathcal{D}|^2\log |\mathcal{C}|}\right)
	\]
\end{prop}
\begin{proof}
	The reduction due to \textcite{BM07} (theorem 18) translates our bound on external regret to a bound on the agent's regret with respect to modification rules $\mathcal{G}$. For any $\vec{r}_0$ and $\pi_{0c}\in\mathcal{D}_{\vec{r}_0}$,
	\begin{align*}
		&(1-\alpha)\sum_{c\in\mathcal{C}}\sum_{i=1}^{n_c}\left(\ex[b,\pi\sim\upsilon_{c_i}]{U(\vec{r}_{0c},p^\dagger(b,\pi),y_{c_i})}-\ex[\vec{r}\sim F]{\ex[b,\pi\sim\upsilon_{c_i}]{U(\vec{r},p^\dagger(b,\pi),y_{c_i})}}\right)\\
		&\:\:\:\:+\alpha\sum_{c\in\mathcal{C}}\sum_{i=1}^{n_c}\left(\ex[p\sim\diamondsuit]{U(\pi_{0c},p,y_{c_i})}-\ex[\vec{r}\sim F]{\ex[\pi\sim\mu_{c_i,\vec{r}}]{\ex[p\sim\diamondsuit]{U(\pi,p,y_{c_i})}}}\right)\\
		&\leq\er{\Delta\mathcal{Y}}+O\left(\sqrt{T|\mathcal{D}|^2\log |\mathcal{C}|}\right)
	\end{align*}
	The loss due to the restriction $\pi_{0c}\in\mathcal{D}_{\vec{r}_0}$ -- as opposed to the unrestricted choice of $\pi_{0c}\in\Pi_{\vec{r}_0}$ -- is at most $\alpha K_\spadesuit\delta T$ by the second part of assumption \ref{A12}. The desired result follows.
\end{proof}
